# Supplementary material for: TempLe: Learning Template of Transitions for Sample Efficient Multi-task RL
Source: arXiv:2002.06659 source file (2021-03-08)
Supplement: Supplementary file 1 [file discuss.tex]

%!TEX root = ../0_aaai2021_multitaskrl_main.tex

\section{Discussion: Potential Extension to Deep RL}
\label{app:deep}

Our TempLe can be extended to large-scale, continuous MDPs. TempLe is essentially estimating the “relative” transition among states due to the permutation operation. For example, TempLe considers the transition from s_1 to s_2 with probability 0.5 to be similar to the transition from s_7 to s_8 with probability 0.5, since the relative state difference is the same. This is equivalent to predicting a “state shift” in a continuous state space, which is s_{t+1} - s_t. In this case, we can use continuous distributions (e.g. Gaussian) to approximately model the state shift, without doing state counting and ranking.

Our extension to continuous space works as follows:
1) use a neural network (NN) to predict the relative state shift: \hat{\delta} \approx s_{t+1} - s_t;
2) approximately model \delta’s using a mixture of Gaussian, for instance. From the trajectories/history, we compute \delta= s_{t+1} - s_t, cluster them (GEN-TT/TT-UPDATE step of TempLe) and use the averaged \bar{\delta} from each Gaussian subpopulation/cluster to improve the prediction of the NN by minimizing MSE(\hat{\delta}, \bar{\delta});
3) use \bar{\delta} to augment the accuracy of \hat{delta} by identifying it into an existing cluster (AUGMENT step in TempLe). As a result, we can learn an accurate prediction model of the environment.

We implemented the above idea on the CartPole (continuous state) and Mujoco Hopper (continuous state, continuous action). We use a 2-layer MLP with 64 nodes per layer. We compare with two baselines: [Baseline 1] directly predicting the absolute next state, and [Baseline 2] predicting the relative state shift without TempLe, as in [3].

We evaluate the performance using the average model losses [MSE(s_{t+1}, \hat{s_{t+1}}) + MSE(r, \hat{r})] after 200 episodes of training. The results below show that our method outperforms both baselines significantly in CartPole and Hopper. We will incorporate these results into our modified version.

Model losses (the lower the better):
--------------------------------
- CartPole: [Baseline 1] 0.05893; [Baseline 2] 0.00160; [Ours] 0.00023
- Hopper: [Baseline 1] 0.90644; [Baseline 2] 0.03982; [Ours] 0.02782
---------------------------------
