# Supplementary material for: TempLe: Learning Template of Transitions for Sample Efficient Multi-task RL
Source: arXiv:2002.06659 source file (2021-03-08)
Supplement: Supplementary file 2 [file fig_mean.tex]

%!TEX root = ../0_aaai2021_multitaskrl_main.tex
% \vspace{-1.5em}
\begin{figure}[!htbp]
\centering
	\begin{subfigure}[t]{0.3\columnwidth}
		\centering
		\input{\fighome/maze/mean_acc_runs20.tex}
	\vspace{-0.4em}
	\caption{Online MTRL}
	\label{sfig:maze_mean}
	\end{subfigure}
	\hfill
	\begin{subfigure}[t]{0.3\columnwidth}
		\centering
		\input{\fighome/group/mean_acc_runs30_abs_maxqint.tex}
		\vspace{-0.4em}
		\caption{Finite-Model MTRL}
		\label{sfig:group_mean}
	\end{subfigure}
	\hfill
	\begin{subfigure}[t]{0.3\columnwidth}
		\centering
		\input{\fighome/var/lifelong-varsize_mean_acc_runs10.tex}
		\vspace{-0.4em}
		\caption{Varying Sized MTRL}
		\label{sfig:var_mean}
	\end{subfigure}
\vspace{-0.5em}
\caption{Mean reward comparison of \ourmod and \ourmodtwo compared against baselines in (a) Online MTRL, (b) Finite-Model MTRL and (c) varying sized MTRL. 
}
\label{fig:mean}
\end{figure}
% \vspace{-0.5em}
