# Supplementary material for: TempLe: Learning Template of Transitions for Sample Efficient Multi-task RL
Source: arXiv:2002.06659 source file (2021-03-08)
Supplement: Supplementary file 3 [file mean_acc_runs30.tex]

% This file was created by matplotlib2tikz v0.7.4.
\begin{tikzpicture}

\definecolor{color0}{rgb}{0.462745098039216,0.654901960784314,0.490196078431373}
\definecolor{color1}{rgb}{0.4,0.470588235294118,0.67843137254902}
\definecolor{color2}{rgb}{0.776470588235294,0.443137254901961,0.443137254901961}

\begin{axis}[
legend cell align={left},
legend style={at={(0.03,0.97)}, anchor=north west, draw=white!80.0!black},
tick align=outside,
tick pos=left,
title={GridWorld},
x grid style={white!69.01960784313725!black},
xlabel={Episodes},
xmajorgrids,
xmin=-236.5, xmax=4988.5,
xtick style={color=black},
y grid style={white!69.01960784313725!black},
ylabel={Cumulative Reward},
ymajorgrids,
ymin=-5638.64316286526, ymax=62759.6013969301,
ytick style={color=black}
]
\path [draw=color0, fill=color0, opacity=0.25]
(axis cs:1,-9.94452498900435)
--(axis cs:1,-7.10880834432899)
--(axis cs:251,-912.159686976111)
--(axis cs:501,-1874.97899143944)
--(axis cs:751,-2231.91462015574)
--(axis cs:1001,1255.52703547789)
--(axis cs:1251,4753.84839421462)
--(axis cs:1501,8255.30382148194)
--(axis cs:1751,11756.7244125734)
--(axis cs:2001,15260.4091857141)
--(axis cs:2251,18763.4026199787)
--(axis cs:2501,22278.308038458)
--(axis cs:2751,25786.4779485943)
--(axis cs:3001,29289.2855711127)
--(axis cs:3251,32793.683556115)
--(axis cs:3501,36300.0331946559)
--(axis cs:3751,39804.3618341089)
--(axis cs:4001,43313.2617171505)
--(axis cs:4251,46818.3027987258)
--(axis cs:4501,50326.5180946248)
--(axis cs:4751,53830.5609019048)
--(axis cs:4751,49277.6657647614)
--(axis cs:4751,49277.6657647614)
--(axis cs:4501,46041.921905375)
--(axis cs:4251,42802.5638679408)
--(axis cs:4001,39575.0449495162)
--(axis cs:3751,36335.7181658913)
--(axis cs:3501,33093.953472011)
--(axis cs:3251,29850.3431105518)
--(axis cs:3001,26618.2077622208)
--(axis cs:2751,23382.7353847392)
--(axis cs:2501,20141.0119615421)
--(axis cs:2251,16895.5307133547)
--(axis cs:2001,13657.1374809526)
--(axis cs:1751,10423.76892076)
--(axis cs:1501,7187.70951185137)
--(axis cs:1251,3955.07160578537)
--(axis cs:1001,717.792964522111)
--(axis cs:751,-2529.63204651093)
--(axis cs:501,-2081.75434189388)
--(axis cs:251,-1071.04031302389)
--(axis cs:1,-9.94452498900435)
--cycle;

\path [draw=color1, fill=color1, opacity=0.25]
(axis cs:1,-8.21642444975097)
--(axis cs:1,0.269757783084298)
--(axis cs:251,2552.15694895375)
--(axis cs:501,5212.87620876359)
--(axis cs:751,8028.87687791523)
--(axis cs:1001,10915.0065861006)
--(axis cs:1251,13827.1936220375)
--(axis cs:1501,16769.4818337862)
--(axis cs:1751,19735.9366601277)
--(axis cs:2001,22723.2739440647)
--(axis cs:2251,25723.8463826652)
--(axis cs:2501,28735.7391099931)
--(axis cs:2751,31764.6163221702)
--(axis cs:3001,34781.689986319)
--(axis cs:3251,37814.7383089887)
--(axis cs:3501,40843.7844629784)
--(axis cs:3751,43885.0164804274)
--(axis cs:4001,46931.8385070384)
--(axis cs:4251,49988.7092323276)
--(axis cs:4501,53036.0080218634)
--(axis cs:4751,56095.9967759471)
--(axis cs:4751,49844.6032240526)
--(axis cs:4751,49844.6032240526)
--(axis cs:4501,47083.898644803)
--(axis cs:4251,44328.7574343389)
--(axis cs:4001,41568.5481596284)
--(axis cs:3751,38830.2901862395)
--(axis cs:3501,36094.6022036885)
--(axis cs:3251,33376.9816910117)
--(axis cs:3001,30645.4033470147)
--(axis cs:2751,27920.0370111634)
--(axis cs:2501,25220.2742233404)
--(axis cs:2251,22526.4069506683)
--(axis cs:2001,19849.0327226021)
--(axis cs:1751,17178.6500065391)
--(axis cs:1501,14509.5048328806)
--(axis cs:1251,11865.5930446292)
--(axis cs:1001,9288.87341389936)
--(axis cs:751,6703.00312208475)
--(axis cs:501,4285.63045790307)
--(axis cs:251,2076.20305104626)
--(axis cs:1,-8.21642444975097)
--cycle;

\path [draw=color2, fill=color2, opacity=0.25]
(axis cs:1,-9.85346993961915)
--(axis cs:1,-6.59986339371419)
--(axis cs:251,-913.825989074009)
--(axis cs:501,96.2647463425179)
--(axis cs:751,3580.1338469402)
--(axis cs:1001,7078.53154574445)
--(axis cs:1251,10578.278610575)
--(axis cs:1501,14085.629772288)
--(axis cs:1751,17586.6739888408)
--(axis cs:2001,21090.2630364808)
--(axis cs:2251,24598.0119261409)
--(axis cs:2501,28108.0475617767)
--(axis cs:2751,31606.5736373571)
--(axis cs:3001,35105.8739161629)
--(axis cs:3251,38612.9780465518)
--(axis cs:3501,42120.3013708744)
--(axis cs:3751,45629.8882315318)
--(axis cs:4001,49134.480909882)
--(axis cs:4251,52637.3035055275)
--(axis cs:4501,56140.4083710412)
--(axis cs:4751,59650.5902805758)
--(axis cs:4751,54839.8897194236)
--(axis cs:4751,54839.8897194236)
--(axis cs:4501,51594.138295625)
--(axis cs:4251,48361.5764944722)
--(axis cs:4001,45126.5857567844)
--(axis cs:3751,41890.2317684682)
--(axis cs:3501,38656.9386291257)
--(axis cs:3251,35420.0619534484)
--(axis cs:3001,32180.9660838374)
--(axis cs:2751,28954.7330293098)
--(axis cs:2501,25728.6991048901)
--(axis cs:2251,22488.6280738593)
--(axis cs:2001,19248.8702968526)
--(axis cs:1751,16015.0326778259)
--(axis cs:1501,12775.9835610454)
--(axis cs:1251,9538.40138942499)
--(axis cs:1001,6306.29512092221)
--(axis cs:751,3063.09281972648)
--(axis cs:501,-180.278079675844)
--(axis cs:251,-1068.36067759266)
--(axis cs:1,-9.85346993961915)
--cycle;

\addplot [semithick, color0, mark=*, mark size=3, mark options={solid}]
table {%
1 -8.52666666666667
251 -991.599999999999
501 -1978.36666666666
751 -2380.77333333333
1001 986.659999999999
1251 4354.46
1501 7721.50666666666
1751 11090.2466666667
2001 14458.7733333334
2251 17829.4666666667
2501 21209.6600000001
2751 24584.6066666667
3001 27953.7466666667
3251 31322.0133333334
3501 34696.9933333334
3751 38070.0400000001
4001 41444.1533333334
4251 44810.4333333333
4501 48184.2199999999
4751 51554.1133333331
};
\addlegendentry{RMax}
\addplot [semithick, color1, mark=square*, mark size=3, mark options={solid}]
table {%
1 -3.97333333333333
251 2314.18
501 4749.25333333333
751 7365.93999999999
1001 10101.94
1251 12846.3933333334
1501 15639.4933333334
1751 18457.2933333334
2001 21286.1533333334
2251 24125.1266666668
2501 26978.0066666668
2751 29842.3266666668
3001 32713.5466666668
3251 35595.8600000002
3501 38469.1933333335
3751 41357.6533333334
4001 44250.1933333334
4251 47158.7333333333
4501 50059.9533333332
4751 52970.2999999998
};
\addlegendentry{Q-learning}
\addplot [semithick, color2, mark=diamond*, mark size=3, mark options={solid}]
table {%
1 -8.22666666666667
251 -991.093333333333
501 -42.0066666666629
751 3321.61333333334
1001 6692.41333333333
1251 10058.34
1501 13430.8066666667
1751 16800.8533333334
2001 20169.5666666667
2251 23543.3200000001
2501 26918.3733333334
2751 30280.6533333334
3001 33643.4200000001
3251 37016.5200000001
3501 40388.62
3751 43760.06
4001 47130.5333333332
4251 50499.4399999998
4501 53867.2733333331
4751 57245.2399999997
};
\addlegendentry{TempLe}
\end{axis}

\end{tikzpicture}
